# Supplementary material for: Newton Methods for Convolutional Neural Networks
Source: arXiv:1811.06100 ancillary file (2018-11-14)
Supplement: Supplementary file 1 [file supplement.pdf]

# Supplementary Materials for "Newton Methods for Convolutional Neural Networks"

**Chien-Chih Wang, Kent Loong Tan, Chih-Jen Lin**
Department of Computer Science, National Taiwan University, Taipei 10617, Taiwan

# I Alternative Method for the Generation of $\phi(Z^{\text{in},i})$

For the alternative method here, we use *MATLAB*'s `im2col` with $s = 1$ and extract a sub-matrix as $\phi(Z^{\text{in},i})$.

We now explain each line of the program. To find $P_\phi^m$, from (9) what we need is to extract elements in $Z^{\text{in},i}$. In line 2, we start with obtaining the linear indices of the first row of $Z^{\text{in},i}$, which corresponds to the first channel of the image. In line 3, we use `im2col` to build $\phi(Z^{\text{in},i})$ under $s = d^{\text{in}} = 1$, though contents of the input matrix are linear indices of $Z^{\text{in},i}$ rather than values. For $\phi(Z^{\text{in},i})$ under $s = d^{\text{in}} = 1$, the matrix size is

$$hh \times \bar{a}\bar{b},$$

where from (4),

$$\bar{a} = a^{\text{in}} - h + 1,\ \bar{b} = b^{\text{in}} - h + 1.$$

From (9), when a general $s$ is considered, we must select some columns, whose column indices are the following subset of $\{1, \ldots, \bar{a}\bar{b}\}$:

$$\mathbb{1}_{b^{\text{out}}} \otimes \left( \begin{bmatrix} 0 \\ \vdots \\ a^{\text{out}} - 1 \end{bmatrix} s + \mathbb{1}_{a^{\text{out}}} \right) + \left( \begin{bmatrix} 0 \\ \vdots \\ b^{\text{out}} - 1 \end{bmatrix} s \right) \otimes \begin{bmatrix} \bar{a} \\ \vdots \\ \bar{a} \end{bmatrix}_{a^{\text{out}} \times 1}, \tag{I.1}$$

where $a^{\text{out}}$ and $b^{\text{out}}$ are defined in (4). More precisely, (I.1) comes from the following mapping between the first row of $\phi(Z^{\text{in},i})$ in (9) and $\{1, \ldots, \bar{a}\bar{b}\}$:

$$\begin{bmatrix} (1,1) \\ (1+s,1) \\ \vdots \\ (1+(a^{\text{out}}-1)s, 1) \\ (1, 1+s) \\ (1+s, 1+s) \\ \vdots \\ (1+(a^{\text{out}}-1)s, 1+s) \\ \vdots \end{bmatrix} \longrightarrow \begin{bmatrix} \begin{bmatrix} 0 \\ \vdots \\ a^{\text{out}} - 1 \end{bmatrix} s + \mathbb{1}_{a^{\text{out}}} + \mathbf{0}_{a^{\text{out}}} s\bar{a} \\ \begin{bmatrix} 0 \\ \vdots \\ a^{\text{out}} - 1 \end{bmatrix} s + \mathbb{1}_{a^{\text{out}}} + \mathbb{1}_{a^{\text{out}}} s\bar{a} \\ \vdots \end{bmatrix}$$

Next we discuss how to extend the linear indices of the first channel to others. From (5), each column of $Z^{\text{in},i}$ contains values of the same pixel in different channels. Therefore, because we consider a column-major order, indices in $Z^{\text{in},i}$ for a given pixel are a

Listing I: An alternative implementation for $\phi(Z^{\text{in},i})$

```
1 function output_idx = find_index_phiZ(a,b,d,h,s)
2     input_idx = reshape(([1:a*b]-1)*d+1,a,b);
3     output_idx = im2col(input_idx,[h,h],'sliding');
4     a_bar = a-h+1;
5     b_bar = b-h+1;
6     a_idx = 1:s:a_bar;
7     b_idx = 1:s:b_bar;
8     select_idx = a_idx'+a_bar*(b_idx-1);
9     output_idx = output_idx(:,select_idx)';
10    output_idx = reshape(output_idx(:)+[0:d-1],[],h*h*d)';
11 end
```

continuous segment. Then in (9) for $\phi(Z^{\text{in},i})$, essentially we have $d^{\text{in}}$ segments ordered vertically and elements in two consecutive segments are from two consecutive rows in $Z^{\text{in},i}$. Therefore, the following index matrix can be used to extract all needed elements in $Z^{\text{in},i}$ for $\phi(Z^{\text{in},i})$.

$$\mathbb{1}_{d^{\text{in}}} \otimes \begin{bmatrix} \text{linear indices of } Z^{\text{in},i} \text{ for} \\ \text{1st channel of } \phi(Z^{\text{in},i}) \end{bmatrix}_{hh \times a^{\text{out}} b^{\text{out}}} + \left( \begin{bmatrix} 0 \\ \vdots \\ d^{\text{in}} - 1 \end{bmatrix} \otimes \mathbb{1}_{hh} \right) \otimes \mathbb{1}^T_{a^{\text{out}} b^{\text{out}}}. \quad \text{(I.2)}$$

The implementation is in line 10. Since *OCTAVE* does not have the function `repelem`,[1] we use different approach to calculate (I.2). First we calculate

$$\text{vec}(\begin{bmatrix} \text{linear indices of } Z^{\text{in},i} \text{ for} \\ \text{1st channel of } \phi(Z^{\text{in},i}) \end{bmatrix}^T) + \begin{bmatrix} 0 & \dots & d^{\text{in}} - 1 \end{bmatrix} \in R^{a^{\text{out}} b^{\text{out}} hh \times d^{\text{in}}}. \quad \text{(I.3)}$$

Then, to obtain the desired matrix, we reshape (I.3) into $R^{a^{\text{out}} b^{\text{out}} \times hhd^{\text{in}}}$ and transpose it.

# II Generation of The Indices in Padding Operations

Assume the input image is

$$Z \in R^{a \times b}.$$

We would like to add $p$ zeros on each dimension so that the resulting image is as Figure II.1. We notice that $Z$ corresponds to the following elements in the output image:

[1] The `repelem` in *MATLAB* is syntax incompatible with the `repelems` in *OCTAVE*.

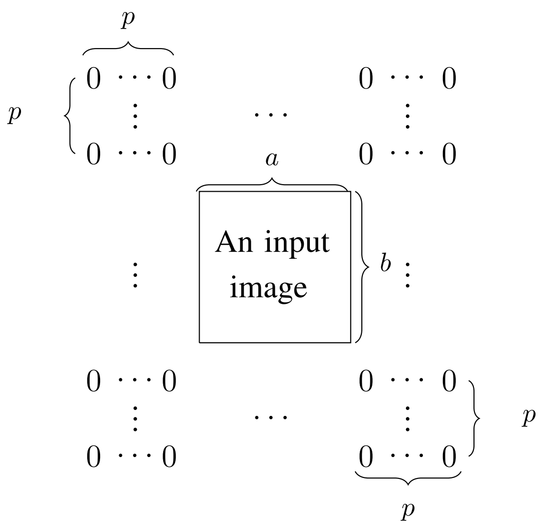


Figure II.1: A padding example.

$$\begin{matrix} (p+1, p+1) & \dots & (p+1, p+b) \\ & \vdots & \\ (p+a, p+1) & \dots & (p+a, p+b) \end{matrix}$$

The size of the new image is

$$(2p+a) \times (2p+b).$$

The linear indices in the new matrix are

$$p\bar{a} + \begin{bmatrix} p+1 \\ \vdots \\ p+a \end{bmatrix}, \ (p+1)\bar{a} + \begin{bmatrix} p+1 \\ \vdots \\ p+a \end{bmatrix}, \ \dots, \ (p+b-1)\bar{a} + \begin{bmatrix} p+1 \\ \vdots \\ p+a \end{bmatrix},$$

where

$$\bar{a} = 2p + a.$$

Together they can be obtained by applying *MATLAB*'s '+' operator on the following two arrays:

$$\begin{bmatrix} p+1 \\ \vdots \\ p+a \end{bmatrix} \text{ and } \bar{a}\begin{bmatrix} p & \cdots & p+b-1 \end{bmatrix}.$$

# III Evaluation of $(\boldsymbol{v}^i)^T P_{\text{pool}}^{m,i}$ in Gradient and Jacobian Evaluations

Because $P_{\text{pool}}^{m,i}$ is similar to $P_{\phi}^{m}$ for mapping linear indices of $Z^{m-1,i}$ to another matrix, the same setting in Section 4.4.1 of using *MATLAB*'s `accumarray` can be applied. The remaining issue is to handle all data together. Here we discuss the calculation of (63) and (67) respectively.

## III.1 Evaluation of $(\boldsymbol{v}^i)^T P_{\text{pool}}^{m,i}$ in Gradient Evaluations

Similar to (104), we calculate

$$\begin{bmatrix} (P_{\text{pool}}^{m,1})^T \boldsymbol{v}^1 \\ \vdots \\ (P_{\text{pool}}^{m,l})^T \boldsymbol{v}^l \end{bmatrix}^T \in R^{d^{m+1} a_{\text{conv}}^m b_{\text{conv}}^m l \times 1}. \tag{III.4}$$

In Section 4.2 we have obtained the linear indices of (82) that correspond to the max values without considering the instance offset

$$(d^{m+1} a_{\text{conv}}^m b_{\text{conv}}^m) i.$$

By adding the instance offset, we have the correct mapping to the linear indices of (82) for the selected max values. In other words, similar to (106), we calculate

$$\begin{aligned} &\text{vec}\left((100) + \mathbb{1}_{d^{m+1}a^{m+1}b^{m+1}} \times \left[0, d^{m+1} a_{\text{conv}}^m b_{\text{conv}}^m, \ldots, (l-1) d^{m+1} a_{\text{conv}}^m b_{\text{conv}}^m\right]\right) \\ =&\text{vec}\left((100)\right) + \begin{bmatrix} 0\mathbb{1}_{d^{m+1}a^{m+1}b^{m+1}} \\ d^{m+1} a_{\text{conv}}^m b_{\text{conv}}^m \mathbb{1}_{d^{m+1}a^{m+1}b^{m+1}} \\ \vdots \\ (l-1) d^{m+1} a_{\text{conv}}^m b_{\text{conv}}^m \mathbb{1}_{d^{m+1}a^{m+1}b^{m+1}} \end{bmatrix} \end{aligned} \tag{III.5}$$

before applying `accumarray`. Note that in Listing 4 we use matrix operations in line 14 to perform the summation in (III.5) and then produce the whole vector in line 31.

## III.2 Evaluation of $\boldsymbol{v}^T P_{\text{pool}}^{m,i}$ in Jacobian Evaluation

We would like to have (67) by calculating

$$\begin{bmatrix} (P_{\text{pool}}^{m,1})^T \boldsymbol{v}_1^1 \\ \vdots \\ (P_{\text{pool}}^{m,1})^T \boldsymbol{v}_{n_{L+1}}^1 \\ \vdots \\ (P_{\text{pool}}^{m,l})^T \boldsymbol{v}_{n_{L+1}}^l \end{bmatrix}^T \in R^{d^{m+1} a_{\text{conv}}^m b_{\text{conv}}^m n_{L+1} l \times 1}, \tag{III.6}$$

where

$$(\boldsymbol{v}_u^i)^T = \left( \frac{\partial \boldsymbol{z}^{L+1,i}}{\partial \text{vec}(Z^{m+1,i})^T} \odot \left( \mathbb{1}_{n_{L+1}} \text{vec}(I[Z^{m+1,i}])^T \right) \right)_{u,:} \in R^{1 \times d^{m+1}a^{m+1}b^{m+1}},$$

$$i = 1, \dots, l, \; u = 1, \dots, n_{L+1},$$

and the subscript "$u,:$" indicates the $u$th row of the matrix. The calculation of (III.6) is the same as the calculation of (109). Thus, similar to (112), we need the following indices as input of `accumarray`:

$$\mathbb{1}_{n_{L+1}} \otimes \text{vec}((100)) + \begin{bmatrix} \mathbf{0}_{d^{m+1}a^{m+1}b^{m+1}} \\ d^{m+1}a^m_{\text{conv}}b^m_{\text{conv}}\mathbb{1}_{d^{m+1}a^{m+1}b^{m+1}} \\ \vdots \\ (n_{L+1}-1)d^{m+1}a^m_{\text{conv}}b^m_{\text{conv}}\mathbb{1}_{d^{m+1}a^{m+1}b^{m+1}} \\ \vdots \\ (n_{L+1}l-1)d^{m+1}a^m_{\text{conv}}b^m_{\text{conv}}\mathbb{1}_{d^{m+1}a^{m+1}b^{m+1}} \end{bmatrix}.$$
